# Supplementary material for: Double InfoGAN for Contrastive Analysis
Source: arXiv:2401.17776 source file (2024-01-31)
Supplement: Supplementary file 1 [file supplement_include.tex]

\begin{center}
    \Large{\textbf{Supplementary Material}}
\end{center}
\section{Ethical Statement}
This paper presents the Double InfoGAN method, which aims to improve the accuracy and interpretability of Contrastive Analysis in various fields, including medical imaging. We acknowledge that the use of medical imaging datasets raises ethical concerns that we discuss in the following. 

Firstly, we ensured that all medical imaging datasets used in our experiments were publicly available, anonimized and ethically sourced. Secondly, we aim at developing a method that improves the quality and interpretability of medical images, potentially leading to better diagnosis and treatment. We recognize that the accuracy and reliability of the generated medical images are crucial for clinical decision-making and that, as already mentioned in the article, more powerful GAN architectures with specific anatomical regularizations will be explored in future. Another ethical concern is the potential for biased outcomes, particularly when the datasets are not representative of the entire population. Biases in the data can lead to inaccurate and unfair results, which could exacerbate healthcare disparities or bring to wrong diagnosis and treatments. Therefore, it is important to ensure that datasets are diverse, inclusive and not biased, representing different demographics, hospitals, conditions, etc. 

In summary, while contrastive analysis can lead to significant improvements in healthcare and in other domains, it is essential to address potential ethical concerns, such as privacy and bias, to ensure accurate and trustworthy results.

\section{Architecture}\label{app:architecture}
We present here the architectures used to obtain the results of this paper. These are inspired by DCGAN \cite{Radford2016}, with the addition of Gaussian Noise in the Discriminator. This prevents it from converging too fast and improves our performances. For the Brats dataset, we also added the spectral norm in the discriminator (instead of the batchnorm), and an attention block in the generator.

All computations are run on a server with one NVIDIA A100 GPU card and 64 AMD EPYC 7302 16-Core Processors.

\begin{table}[h!]
\begin{center}
\begin{adjustbox}{max width=\textwidth}
\begin{tabular}{|l| l |}
\hline
Discriminator D / C / Q & Generator G \\
\hline
Input $64\times 64 \times c $ ; c=3 for RGB, c=1 for gray/binary & Input  $ z \in \mathbb{R}^n, s \in \mathbb{R}^m $ \\

Gaussian noise, $4\times4$ conv 64, stride 2, lReLU & concat and reshape $(z+s,1,1)$ \\
Gaussian noise, $4\times4$ conv 128, stride 2, batchnorm, lReLU & $4 \times 4$ convtranspose 512, batchnorm, ReLU \\
Gaussian noise, $4\times4$ conv 256, stride 2, batchnorm, lReLU & $4 \times 4$ convtranspose 256, stride 2, batchnorm, ReLU  \\
Gaussian noise, $4\times4$ conv 512, stride 2, batchnorm, lReLU (*) & $4 \times 4$ convtranspose 128, stride 2, batchnorm, ReLU  \\
From *:  Gaussian noise, $4\times4$ conv 1, sigmoid (output layer for D) & $4 \times 4$ convtranspose 64, stride 2, batchnorm, ReLU  \\
From *:  Gaussian noise, $4\times4$ conv 1, sigmoid (output layer for C) &  $4 \times 4$ convtranspose c , stride 2, Tanh  \\
From *: Gaussian noise, $4\times4$ conv n (output layer for $Q_z$) & \\
From *: Gaussian noise, $4\times4$ conv m (output layer for $Q_s$) & \\
\hline
\end{tabular}
\end{adjustbox}
\end{center}
\caption{Architecture for celeba, cifar/mnist and dsprite/mnist datasets. Gaussian Noise is added at every layer, with standard deviation of 0.2. LeakyReLU has a negative slope of 0.2. Batch size of 128. When a CR module is added, it has the same architecture as $Q_s$}
\end{table}

\begin{table}[h!]
\begin{center}
\begin{adjustbox}{max width=\textwidth}
\begin{tabular}{|l| l |}
\hline
Discriminator D / C / Q & Generator G \\
\hline
Input $128\times 128 \times 1 $ & Input  $ z \in \mathbb{R}^n, s \in \mathbb{R}^m $ \\

Gaussian noise, $4\times4$ conv 64, stride 2, spectral norm, lReLU & concat + FC $8192$ +reshape $(512,4,4)$ \\
Gaussian noise, $4\times4$ conv 128, stride 2, spectral norm, lReLU & upsample, $3 \times 3$ conv 1024, batchnorm, ReLU \\
Gaussian noise, $4\times4$ conv 256, stride 2, spectral norm, lReLU &  upsample, $3 \times 3$ conv 512, batchnorm, ReLU  \\
Gaussian noise, $4\times4$ conv 512, stride 2, spectral norm, lReLU &  upsample, $3 \times 3$ conv 256, batchnorm, ReLU \\
Gaussian noise, $4\times4$ conv 512, stride 2, spectral norm, lReLU (*) & Self-Attention Block  \\
From *:  Gaussian noise, FC $1$, sigmoid (output layer for D) &upsample, $3 \times 3$ conv 256, batchnorm, ReLU  \\
From *:  Gaussian noise, FC 1, sigmoid (output layer for C) & $3 \times 3$ conv 128, batchnorm, ReLU \\
From *: Gaussian noise, FC 128 , spectral norm, lReLU &  upsample, $3 \times 3$ conv 64, batchnorm, ReLU  \\
Gaussian noise, FC n , spectral norm, lReLU (output layer for $Q_z$) &  $3 \times 3$ conv 1, tanh \\
From *: Gaussian noise , FC 128 , SN, lReLU & \\
Gaussian noise, FC m , spectral norm, lReLU (output layer for $Q_s$) & \\
\hline
\end{tabular}
\end{adjustbox}
\end{center}
\caption{Architecture for Brats. Gaussian noise is additive, with standard deviation of 0.2. LeakyReLU has a negative slope of 0.2. Batch size of 32.}
\end{table}
\newpage

\section{Mathematical developments}\label{app:math}
\subsection{InfoGAN and InfoGAN-CR}\label{app:InfoGAN}
The regularization loss proposed in InfoGAN \cite{chen_infogan_2016} is:

\begin{equation}
\begin{split}
 &I(\bc;\bx) = -H(\bc|\bx) + H(\bc) = \bbE_{\bx \sim P(\bx), \bc \sim P(\bc|\bx)} \log P(\bc|\bx) + H(\bc)= \\
 &=\int P(\bx) \int P(\bc|\bx)  \log(P(\bc|\bx)) dx dc + H(\bc) =\\
&=\int P(\bx) \int P(\bc'|\bx)  \log(P(\bc'|\bx)) dx dc' + H(\bc') = \quad \text{(change of variables between c and c')}\\
&=\int \int \int P(\bx, \bc, \bz) dc dz \int P(\bc'|\bx)  \log(P(\bc'|\bx)) dx dc' + H(\bc') =\\
&=\int P(\bz) \int P(\bc) \int P(\bx|\bc, \bz) \int P(\bc'|\bx)  \log(P(\bc'|\bx)) dz dx dc' dc + H(\bc') =\\
&=\int P(\bz) \int P(\bc) \int P(\bx|\bc, \bz) \int P(\bc'|\bx)  \log(P(\bc'|\bx) \frac{Q(\bc'|\bx)}{Q(\bc'|\bx)}) dz dx dc' dc + H(\bc') = \quad \text{(identity trick)}\\
 &= \underbrace{\bbE_{\bz \sim P(\bz), \bc \sim P(\bc),\bx \sim P(\bx |\bc, \bz)} KL(P(\bc'|\bx) || Q(\bc'|\bx))}_{\geq 0} + \bbE_{\bz \sim P(\bz), \bc \sim P(\bc),\bx \sim P(\bx |\bc, \bz)} \bbE_{c' \sim P(\bc'|\bx)} \log Q(\bc'|\bx) + H(\bc')\\
 &\geq  \bbE_{\bz \sim P(\bz), \bc \sim P(\bc),\bx \sim P(\bx |\bc, \bz)} \bbE_{\bc' \sim P(\bc'|\bx)} \log( Q(\bc'|\bx)) + H(\bc')
 \label{app:InfoGAN-I}
\end{split}
\end{equation}

where we have introduced an auxiliary distribution $Q(\bc|\bx)$, parameterized as a neural network, to approximate the posterior $P(\bc|\bx)$ (which is difficult to compute) and we have made the hypothesis that $\bc$ does not depend on $\bz$ (i.e., $P(\bc|\bz)=P(\bc)$). To further remove also the need to sample from $P(\bc|\bx)$ (which would be impossible in most cases), authors propose a simple, yet effective, modification of the previous variational lower bound. In their algorithm, they actually compute and maximize: $\cL(G,Q) = \bbE_{\bz \sim P(\bz), \bc \sim P(\bc),x \sim P(\bx |\bc, \bz)} \log(Q(\bc|\bx)) + H(\bc)$, which is equivalent to the previous lower bound:

\begin{equation}
\begin{split}
&\cL(G,Q) = \bbE_{\bz \sim P(\bz), \bc \sim P(\bc),\bx \sim P(\bx |\bc, \bz)} \log(Q(\bc|\bx)) + H(\bc)=\\
&= \int P(\bz) \int P(\bc) \int P(\bx |\bc,\bz) \log(Q(\bc|\bx)) dz dc dx + H(\bc)=\\
&= \int P(\bz) \int \int  P(\bx, \bc|\bz) \log(Q(\bc|\bx)) dz dc dx + H(\bc)=\\
&= \int P(\bz) \int \int  P(\bx, \bc'|\bz) \log(Q(\bc'|\bx)) dz dc' dx + H(\bc')= \quad \text{(change of variable between c and c')}\\
&=\int P(\bz) \int \int  P(\bx | \bz) P(\bc'|\bx,\bz)  \log(Q(\bc'|\bx)) dz dc' dx + H(\bc')=\\ 
&=\int P(\bz) \int \int \int P(\bx, \bc | \bz) P(\bc'|\bx)  \log(Q(\bc'|\bx)) dz dc' dx dc + H(\bc') = \quad \text{(c' does not depend on z and re-introduce c)}\\
&=\int P(\bz) \int \int \int P(\bc) P(\bx |\bc, \bz) P(\bc'|\bx)  \log(Q(\bc'|\bx)) dz dc' dx dc + H(\bc') =\\
 &= \bbE_{\bz \sim P(\bz), \bc \sim P(\bc),\bx \sim P(\bx |\bc, \bz)} \bbE_{\bc' \sim P(\bc'|\bx)} \log(Q(\bc'|\bx)) + H(\bc')
 \label{app:InfoGAN-loss}
\end{split}
\end{equation}

In \cite{chen_infogan_2016}, authors proposed to model the auxiliary conditional distribution $Q(\bc|\bx)$ as a \textit{factorized Gaussian} with \textit{identity covariance} $Q(\bc|\bx) = 
 \prod_i (c_i|\bx) = \prod_i  \cN(\mu_i(\bx), 1)$. As shown in \cite{Lin2020}, this is fundamental for stability and efficiency. Furthermore, in \cite{Lin2020}, authors also showed that informativeness alone does not necessarily encourage disentanglement. To this end, they propose a new regularizer, called \textit{Contrastive Regularizer} (CR), which enforces distinguishable visual changes in the images created using different latent codes. More specifically, they propose to fix a latent code $c_i$, draw the others $\{ c_j \}_{j \neq i}$ uniformly at random, and then sample two or more images $x_i$ from the resulting distribution $(x_i) \sim Q^i$. By repeating this process for all $k$ latent codes $c_i$, one can obtain an estimate of all distributions $Q^i$. The goal, following the usual definition of disentanglement, is then to maximize the difference between the distributions $Q^i$, so that each latent code $c_i$ should encode a specific visual variation in the created images that should be noticeable and easy to distinguish from the patterns encoded by the other latent codes $\{ c_j \}_{j \neq i}$. 
 Authors propose to maximize the following loss:

 \begin{equation}
  \cL_c = d_{JS}(Q^1,...,Q^k) := \frac{1}{k} \sum_i KL(Q^i || \frac{\sum_{j} Q^j}{k})   
 \end{equation}

They propose to approximate this regularization term using a discriminator $H$ that performs multi-way hypothesis testing. Given two or more images $(x_i)$, created by fixing only one latent code $c_i$, the discriminator $H$ needs to identify the latent dimension $i$ shared between the images. Authors claim, and experimentally demonstrate, that by updating both discriminator $H$ and generator $G$ to maximize $\cL_c$ it "should encourage each latent code $c_i$ to make distinct and noticeable changes, hence promoting disentanglement". 

We adapted the CR module for our model, as explained in Fig.\ref{fig:cr}.

\begin{figure}[h]
    \centering
\includegraphics[width=14cm]{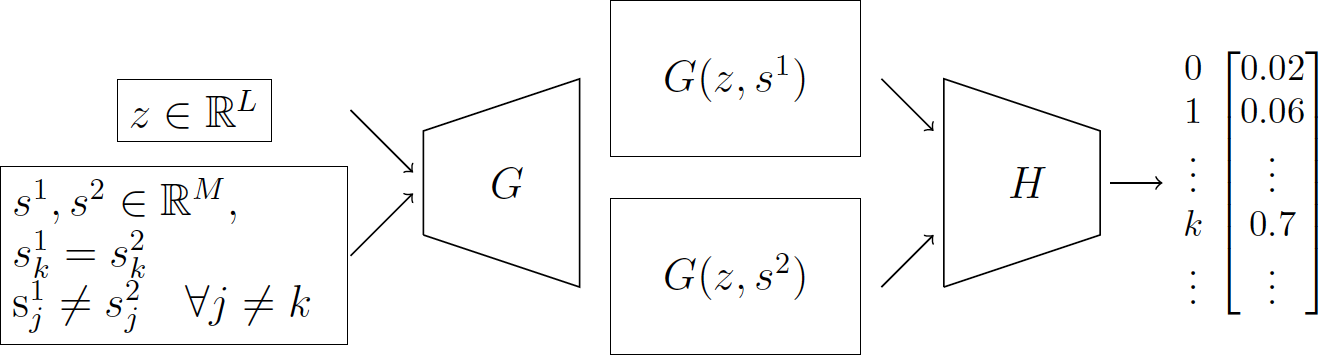}
\caption{Contrastive regularizer. Two images are generated with the following constraints: the background latent space $z$ is the same, and all the salient latent code are different except one (named $k$ here). From these two images, the CR module is then trained to predict which one of the latent code was identical. The CR module outputs a vector of probabilities of the same size as $s$.}
    \label{fig:cr}
\end{figure}

\subsection{Double InfoGAN}\label{app:DoubleINFOGAN}

Since $\bz$ and $\bs$ are supposed to be independent, the mutual information $I((\bz,\bs); \by)$ can be decomposed into the sum of the two mutual information $I(\bz; \by) + I(\bs ; \by)$

\begin{equation}
\begin{split}
 &I((\bz, \bs);\by) = -H((\bz, \bs) | \by) + H(\bz , \bs) = -H((\bz, \bs) | \by) + H(\bz) + H(\bs)=\\
 &= \int \int \int P(\bz , \bs , \by) \log(\frac{P(\bz , \bs , \by)}{P(\by)}) dz ds dy + H(\bz) + H(\bs)=\\
 &= \int P(\by) \int \int P(\bs | \by) P(\bz|\by)  \log(P(\bs | \by) P(\bz|\by) ) dz ds dy + H(\bz) + H(\bs)= \quad \text{(suppose $P(\bs,\bz|\by)=P(\bs | \by) P(\bz|\by) )$}\\
 &= \int P(\by) \int \int P(\bs | \by) P(\bz|\by) \left( \log(P(\bs | \by)) + \log(P(\bz|\by) ) \right) dz ds dy + H(\bz) + H(\bs)=\\
 &= \int_y P(\by) \left ( \int_s P(\bs | \by) \log(P(\bs | \by)) + \int_z P(\bz|\by) \log(P(\bz|\by) )\right) dz ds dy + H(\bz) + H(\bs)=\\
 &=\bbE_{\by \sim P(\by), \bs \sim P(\bs | \by)} \log(P(\bs | \by) + \bbE_{\by \sim P(\by), \bz \sim P(\bz | \by)} \log(P(\bz | \by) + H(\bz) + H(\bs)=\\
 &= -H(\bs | \by) - H(\bz | \by) + H(\bz) + H(\bs) = I(\bz; \by) + I(\bs ; \by)
 \label{eq:DoubleInfoGAN}
\end{split}
\end{equation}

The log-likelihood $\log(P(y))$ of the generated images based on the proposed model is:

\begin{equation}
\begin{split}
 &\log P(\by) = \log \int \int \int P(\by,\bz,\bs,\by_R) dz ds dy_R = \log \int \int \int P(\by|\bz,\bs,\by_R) P(\bz,\bs|\by_R) P(\by_R) \frac{Q(\bz,\bs|\by_R)}{Q(\bz,\bs|\by_R)} dz ds dy_R\\
 &= \log \bbE_{\by_R \sim P(\by_R), (\bz,\bs) \sim Q(\bz, \bs |\by_R)} P(\by|\bz,\bs,\by_R)\frac{P(\bz,\bs|\by_R)}{Q(\bz,\bs|\by_R)} \geq \bbE_{\by_R \sim P(\by_R), (\bz,\bs) \sim Q(\bz, \bs |\by_R)} \log P(\by|\bz,\bs,\by_R)\frac{P(\bz,\bs|\by_R)}{Q(\bz,\bs|\by_R)}=\\
 &= \bbE_{\by_R \sim P(\by_R), (\bz,\bs) \sim Q(\bz, \bs |\by_R)} \log P(\by|\bz,\bs,\by_R) - \bbE_{\by_R \sim P(\by_R)} KL(Q(\bz,\bs|\by_R) || P(\bz,\bs|\by_R))
\end{split}
\end{equation}

\section{Losses equations}\label{app:loss}

In this section, we detail the different losses used in our paper as functions of the involved modules: discriminator, generator, encoder.
%In the following we write these functions for the generator and the discriminator separately, so that the indicated functions are to be minimized. 
Notation are as follows : from an image $I$, $D(I)$ will be the standard adversarial output of the GAN discriminator (namely the probability that an image is real or fake), $C(I)$ will be the class predicted by the discriminator from image $I$, and $Q(I)$ will be the predicted $\hat{z}$ and $\hat{s}$. In practice, Q, C and D share most of the layers (see detailed architecture). 

Reminder of the global loss : 

\begin{equation}
\label{eq:cr}
\begin{split}
    \underset{G,Q,H,C}{min} \underset{D}{max} \quad w_{Adv}  \cdot \mathcal{L}_{Adv}(G,D) +  w_{Class} \cdot \mathcal{L}_{Class}(G,C) \\ 
    + w_{Info}  \cdot \mathcal{L}_{Info}(G,Q) 
    + w_{Im} \cdot \mathcal{L}_{Im}(G,Q) \\
    + w_{CR}  \cdot \mathcal{L}_{CR}(G,H)
\end{split}
\end{equation}

\subsection{Adversarial GAN Loss}\label{app:eq-Adv}
Similarly to \cite{Goodfellow2014}, the adversarial loss used here is: 
\begin{equation}
\begin{split}
    \mathcal{L}_{Adv}(D,G) = w_{bg}  \Bigl( - \mathbb{E}_{\bx_R\sim P(\bx_R)}\bigl[\log(D(\bx_R)\bigr] - 
    \mathbb{E}_{z \sim P_x(\bz)}\bigl[\log(1-(D(G(\bz,0))))\bigr] \Bigr) \\
    w_t \Bigl( - \mathbb{E}_{\by_R\sim P(\by_R)}\bigl[\log(D(\by_R)\bigr] 
    - \mathbb{E}_{\bz,\bs \sim P_y(\bz,\bs)}\bigl[\log(1-(D(G(\bz,\bs))))\bigr]\Bigr)
\end{split}
\end{equation}

%\begin{equation}
%    \mathcal{L}_{NSGAN}^G = - w_{bg}\cdot\mathbb{E}_{z\sim \mathcal{N}(0,1)}%[\log(D(G(z,0))] - w_t \cdot \mathbb{E}_{z,s\sim \mathcal{N}(0,1)}[\log(D(G(z,s))] 
%\end{equation}

%\subsection{Class Loss}

%Labels for class X (resp. Y) are arbitrarily 0 (resp. 1). We use the binary cross entropy (BCE). The discriminator $C$ is trained on real images only to distinguish background images X from target images Y, and the generator is trained using the output of C. The generator is trained so that the images $G(z,0)$ are labeled 0, as the images of the background X, and that the images $G(z,s)$ are labeled 1, as the target images of Y.

%\begin{equation}
%    \mathcal{L}_{class}^{C} = w_{bg} \mathbb{E}_{\bx_R\sim P(\bx_R)}\bigl[BCE(C(\bx_R), 0)\bigr] +  w_t  \mathbb{E}_{\by_R\sim P(\by_R)}\bigl[BCE(C(\by_R), 1)\bigr]
%\end{equation}

%\begin{equation}
%    \mathcal{L}_{Class}^G = w_{bg} \mathbb{E}_{z\sim \mathcal{N}(0,1)}[BCE(C(G(z,0)), 1)] + w_t \cdot \mathbb{E}_{z,s \sim \mathcal{N}(0,1)}[BCE(C(G(z,s)), 0)]
%\end{equation}

\subsection{Info Loss}

%The info loss is the same for the generator G and the output Q of the discriminator, the goal being always to reconstruct z and s, similarly to InfoGAN. However, here we have also added another term for Q.  When a real background image $I_X$ is used, we also want $Q_s(I_X)$ to be zero. 
The weight $w_{Info}$ is actually divided in three components : $w_{Info}^s$, $w_{Info}^z$ and $w_{Info}^{real}$

\begin{equation}
\begin{split}
    \mathcal{L}_{Info}(G,Q) &= w_{bg} \mathbb{E}_{\bz \sim P_y(\bz)}\bigl[w_{Info}^z |(Q_z(G(z,0))- z| + w_{Info}^s |Q_s(G(z,0))- 0|\bigr]\\
    &+ w_t \mathbb{E}_{\bz,\bs \sim P_y(\bz,\bs)}\bigl[w_{Info}^z  |(Q_z(G(z,s))- z| + w_{Info}^s |Q_s(G(z,s))- s|\bigr]\\& +  w_{Info}^{real} \mathbb{E}_{\bx_R \sim P(\bx_R)}\bigl[|(Q_s(\bx_R))- 0|\bigr]
\end{split}
\end{equation}

\subsection{Image reconstruction loss}
We also use an image reconstruction loss, which depends on G and Q: 

\begin{equation}
    \mathcal{L}_{Im}(G,Q) = w_{bg} \mathbb{E}_{ \bx_R \sim P(\bx_R), \hat{z}=Q_z(\bx_R)}\bigl[|G(\hat{z},0) - \bx_R|\bigr] +  w_t \mathbb{E}_{\by_R \sim P(\by_R), \hat{z}, \hat{s}=Q(\by_R)}\bigl[|G(\hat{z},\hat{s}) - \by_R|\bigr]
\end{equation}

\subsection{CR Loss}\label{app:CR-loss}

The Contrastive Regularization loss is computed to improve the disentanglement of $\bs$. The module H and the generator G are trained using a Cross Entropy loss to find the salient feature $k$ in common between two images generated with two salient factors that have only one factor in common (i.e., $s^1_k = s^2_k$) and all other factors different (i.e., $s^1_j \neq s^2_j$ with $\forall j \neq k$):

\begin{equation}
    \mathcal{L}_{CR}(G,H) = \mathbb{E}_{k \in \mathbb{N}, z \sim P_y(\bz), s^1,s^2 \sim P_y(\bs), s^1_k = s^2_k, s^1_j \neq s^2_j, \forall j \neq k}\Bigl[CE\bigl(H(G(z,s^1), G(z,s^2)), k\bigr)\Bigr]
\end{equation}

\subsection{Weights and ratio between the losses}
Different weights are used to balance the different losses, as well as other hyper-parameters (learning rate, number of epochs, etc.). Table~\ref{tab:weights} summarizes the hyper-parameters used in our experiments and their values for each dataset employed. %for the purpose of reproducibility

\begin{table}
    \centering
    \begin{tabular}{c|c|c|c|c|c}
 \multirow{2}{*}{parameters}  &  \multirow{2}{*}{definition} &  \multicolumn{4}{c}{value for different datasets} \\
&  & celeba & cifar-mnist  & mnist-dsprite & brats\\
\hline
loop G  & number of G loop & 1 & 1 & 2 & 1 \\
loop D  & number of D loop & 1 & 1 & 1 & 1 \\
loop CR (when used) & number of CR loop & - & 1 & 1 & 1 \\
lr G    & learning rate G & 0.0002 & 0.0002 & $5\cdot 10^{-5}$ & 0.0001\\
lr D    & learning rate D & 0.0002 & 0.0002 & $5\cdot 10^{-5}$ & 0.0001\\
lr CR  (when used) & learning rate CR & - & 0.0002 & $5\cdot 10^{-5}$ & 0.0001\\
$w_{bg}$& weight for background & 0.5 & 0.5 & 0.5 & 0.5\\
$w_t$   & weight for target losses & 1.0 & 1.0 & 1.0 & 1.0\\
$w_{Adv}$ & weight for adversarial loss & 0.5 & 0.5 & 0.5 & 0.5\\
$w_{Class}$ & weight for class classification & 0.5 & 0.5 & 0.5 & 0.5\\
$w_{Image}$ & weight for image reconstruction & 1.0 & 1.0 & 1.0 & 1.0\\
$w_{Info}^z$ & weight for info loss z & 1.0 & 1.0 & 1.0 & 1.0\\
$w_{Info}^s$ & weight for info loss s & 1.0 & 1.0 & 1.0 & 1.0 \\
$w_{Info}^{real}$ & weight for info loss real image & 1.0 & 1.0 & 1.0 & 1.0 \\
$w_{CR}$ (when used) & weight for CR loss & - & 1.0 & 1.0 & 1.0\\
    \end{tabular}
    \caption{Hyperparameters used for every dataset}
    \label{tab:weights}
\end{table}

\section{Extensive Results}\label{app:extensive-results}

\begin{table}
    \centering
    \begin{tabular}{c|c c | c c }
    original images &  \multicolumn{2}{c|}{Image reconstruction}  &  \multicolumn{2}{c}{Image swap} \\
                        & MM-cVAE & double InfoGAN & MM-cVAE & double InfoGAN \\
        \includegraphics[width=2cm]{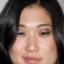} & \includegraphics[width=2cm]{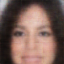} & \includegraphics[width=2cm]{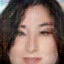} & \includegraphics[width=2cm]{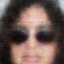} & \includegraphics[width=2cm]{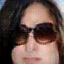} \\
        \includegraphics[width=2cm]{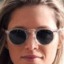} & \includegraphics[width=2cm]{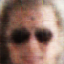} & \includegraphics[width=2cm]{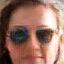} & \includegraphics[width=2cm]{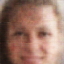} & \includegraphics[width=2cm]{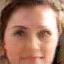} \\
        \hline \\
        \includegraphics[width=2cm]{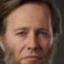} & \includegraphics[width=2cm]{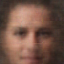} & \includegraphics[width=2cm]{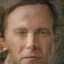} & \includegraphics[width=2cm]{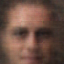} & \includegraphics[width=2cm]{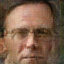} \\
        \includegraphics[width=2cm]{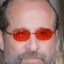} & \includegraphics[width=2cm]{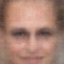} & \includegraphics[width=2cm]{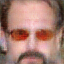} & \includegraphics[width=2cm]{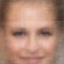} & \includegraphics[width=2cm]{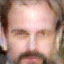} \\
        \hline \\
        \includegraphics[width=2cm]{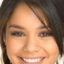} & \includegraphics[width=2cm]{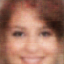} & \includegraphics[width=2cm]{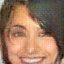} & \includegraphics[width=2cm]{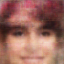} & \includegraphics[width=2cm]{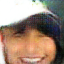} \\
        \includegraphics[width=2cm]{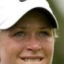} & \includegraphics[width=2cm]{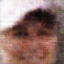} & \includegraphics[width=2cm]{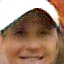} & \includegraphics[width=2cm]{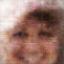} & \includegraphics[width=2cm]{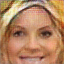} \\
    \end{tabular}
    \captionof{figure}{Image reconstruction and swap with CelebA. In every block, first row refers to $X$ and second row to $Y$. It's interesting to notice that rare attributes, such as the glasses in the first two blocks, are correctly reconstructed by our method and not by MM-cVAE. However, they are changed towards  more "common" glasses after swapping.}
    \label{tab:my_label}
\end{table}

\begin{table}
\begin{center}
\begin{tabular}{|c |cc |cc |cc  | c c |c c |} 
\hline
&  \multicolumn{10}{|c|}{cVAE}   \\ 
& \multicolumn{2}{c|}{epoch 100}   & \multicolumn{2}{c|}{epoch 200} & \multicolumn{2}{c|}{epoch 300} & \multicolumn{2}{c|}{epoch 400} & \multicolumn{2}{c|}{epoch 500} \\
& $s_x$ $\uparrow$ & $z_x$ $\downarrow$ & $s_x$ $\uparrow$ & $z_x$ $\downarrow$ & $s_x$ $\uparrow$ & $z_x$ $\downarrow$ & $s_x$ $\uparrow$ & $z_x$ $\downarrow$& $s_x$ $\uparrow$ & $z_x$ $\downarrow$ \\

Training 1  & $0.81$ & $0.80$ & $0.82$ & $0.80$ & $0.83$ & $0.80$ & $0.82$ & $0.79$ & $0.83$ & $0.80$  \\
Training 2  & $0.78$ & $0.82$ & $0.80$ & $0.82$ & $0.79$ & $0.82$ & $0.80$ & $0.81$ & $0.81$ & $0.81$ \\
Training 3  & $0.79$ & $0.82$ & $0.79$ & $0.82$ & $0.80$ & $0.81$ & $0.81$ & $0.81$ & $0.81$ & $0.81$ \\
Training 4 & $0.83$ & $0.79$ & $0.84$ & $0.78$ & $0.83$ & $0.78$ & $0.84$ & $0.78$ & $\mathbf{0.84}$ & $\mathbf{0.78}$ \\
Training 5 & $0.79$ & $0.82$ & $0.80$ & $0.81$ & $0.82$ & $0.81$ & $0.81$ & $0.80$ & $0.82$ & $0.80$ \\
 \hline
&  \multicolumn{10}{|c|}{MM-cVAE}   \\ 
& \multicolumn{2}{c|}{epoch 100}   & \multicolumn{2}{c|}{epoch 200} & \multicolumn{2}{c|}{epoch 300} & \multicolumn{2}{c|}{epoch 400} & \multicolumn{2}{c|}{epoch 500} \\
& $s_x$ $\uparrow$ & $z_x$ $\downarrow$ & $s_x$ $\uparrow$ & $z_x$ $\downarrow$ & $s_x$ $\uparrow$ & $z_x$ $\downarrow$ & $s_x$ $\uparrow$ & $z_x$ $\downarrow$& $s_x$ $\uparrow$ & $z_x$ $\downarrow$ \\

Training 1 & $0.84 $ & $0.75 $ & $0.84 $ & $0.75$ & $0.85 $ & $0.73$ & $0.85$ & $0.73 $ & $\mathbf{0.85}$ & $\mathbf{0.72}$ \\
Training 2 & $0.83$ & $0.77$ & $0.84$ & $0.76$ & $0.85$ & $0.75$ & $0.85$ &$0.75$ & $0.85$ & $0.74$ \\ 
Training 3 & $nan$ & $nan$ & $nan$ & $nan$ & $nan$ & $nan$ & $nan$ & $nan$ & $nan$ & $nan$ \\
Training 4 &$0.79$& $0.82$ & $0.80$& $0.83$ & $0.73$ & $0.83$ & $0.74$ & $0.83$ & $0.74 $ & $0.83 $ \\
Training 5 & $0.81$ & $0.79$ & $0.82$ & $0.79$ & $0.82$ & $0.79$ & $0.83$ & $0.78$ & $0.83 $ & $0.77 $ \\

 \hline

 &  \multicolumn{10}{|c|}{double InfoGAN}  \\
%  & \multicolumn{2}{c|}{epoch 100}   & \multicolumn{2}{c|}{epoch 200} & \multicolumn{2}{c|}{epoch 300} & \multicolumn{2}{c|}{epoch 400} & \multicolumn{2}{c|}{epoch 500} \\
% & $s_x$ $\uparrow$ & $z_x$ $\downarrow$ & $s_x$ $\uparrow$ & $z_x$ $\downarrow$ & $s_x$ $\uparrow$ & $z_x$ $\downarrow$ & $s_x$ $\uparrow$ & $z_x$ $\downarrow$& $s_x$ $\uparrow$ & $z_x$ $\downarrow$ \\

% Training 1 & $0.87$ & $0.78$ & $0.90$ & $0.73$ & $0.92$ & $0.73$ & $0.93$ & $0.74$ & $0.93 $ & $0.72 $\\
% Training 2 & $0.87$ & $0.80$ & $0.89$ & $0.77$ & $0.90$ & $0.73$ & $0.91$ & $0.77$ &  $0.92 $ & $0.72$ \\
% Training 3 & $0.89$ & $0.84$ & $0.90$ & $0.74$ & $0.91$ & $0.74$ & $0.93$ & $0.74$ &  $0.93 $ & $0.72 $ \\
% Training 4 & $0.85$ & $0.82$ & $0.89$ & $0.75$ & $0.91$ & $0.74$ & $0.92$ & $0.73$ & $\mathbf{0.93}$ & $\mathbf{0.71}$ \\
% Training 5 & $0.78$ & $0.80$ & $0.78$ & $0.81$ & $0.79$ & $0.80$ & $0.81$ & $0.81$ & $0.83$ & $0.79$ \\
% \hline
%  &  \multicolumn{10}{|c|}{double InfoGAN (no CR)}  \\
 & \multicolumn{2}{c|}{epoch 100}   & \multicolumn{2}{c|}{epoch 200} & \multicolumn{2}{c|}{epoch 300} & \multicolumn{2}{c|}{epoch 400} & \multicolumn{2}{c|}{epoch 500} \\

& $s_x$ $\uparrow$ & $z_x$ $\downarrow$ & $s_x$ $\uparrow$ & $z_x$ $\downarrow$ & $s_x$ $\uparrow$ & $z_x$ $\downarrow$ & $s_x$ $\uparrow$ & $z_x$ $\downarrow$& $s_x$ $\uparrow$ & $z_x$ $\downarrow$ \\

Training 1 & $0.93$ & $0.74$ & $0.93$ & $0.73$ & $0.95$ & $0.72$ & $0.95$ & $0.73$ & $0.94$ & $0.70$\\
Training 2 & $0.92$ & $0.70$ & $0.94$ & $0.73$ & $0.95$ & $0.73$ & $0.95$ & $0.74$ & $0.95$ & $0.73$\\
Training 3 & $0.92$ & $0.69$ & $0.94$ & $0.71$ & $0.95$ & $0.74$ & $0.95$ & $0.73$ & $\mathbf{0.95}$ & $\mathbf{0.69}$\\
Training 4 & $0.93$ & $0.72$ & $0.94$ & $0.70$ & $0.95$ & $0.72$ & $0.95$ & $0.71$ & $0.95$ & $0.72$ \\
Training 5 & $0.93$ & $0.72$ & $0.94$ & $0.70$ & $0.95$ & $0.72$ & $0.95$ & $0.76$ & $0.95$ & $0.73$ \\
\hline
\end{tabular}
\end{center}
\caption{Target Dataset separation on CelebA - glasses vs hat - for the 5 trainings of the three methods at different epochs. For clarity, we don't report the standard deviations, whose values are between 0.00 and 0.01. We can notice that the trainings of MMc-VAE are less stable than the ones of our method.}
\label{tab:target-sep-celeba2}
\end{table}

\begin{table}
\begin{center}
\begin{tabular}{|c |cccc |cccc  |cccc|} 
\hline
 &  \multicolumn{12}{|c|}{MM-cVAE with latent space size $128$ $(64\times 2)$}  \\
 
 & \multicolumn{4}{c|}{epoch 100}   & \multicolumn{4}{c|}{epoch 300} & \multicolumn{4}{c|}{epoch 500} \\
 
 & \multicolumn{2}{c|}{Mnist (salient)} & \multicolumn{2}{c|}{Cifar (bg)} 
 & \multicolumn{2}{c|}{Mnist (salient)} & \multicolumn{2}{c|}{Cifar (bg)} 
 & \multicolumn{2}{c|}{Mnist (salient)} & \multicolumn{2}{c|}{Cifar (bg)}\\
 & $s_y$ $\uparrow$ & $z_y$ $\downarrow$  & $s_y$ $\downarrow$ & $z_y$ $\uparrow$ 
 & $s_y$ $\uparrow$ & $z_y$ $\downarrow$  & $s_y$ $\downarrow$ & $z_y$ $\uparrow$ 
 & $s_y$ $\uparrow$ & $z_y$ $\downarrow$  & $s_y$ $\downarrow$ & $z_y$ $\uparrow$ \\ 
 
Training 1  & $0.68$ & $0.57$ & $0.16$ & $0.36$ & $0.68$ & $0.51$ & $0.15$ & $0.36$ & $0.70$ & $0.49$ & $0.16$ & $0.36$ \\
Training 2  & $0.80$ & $0.51$ & $0.15$ & $0.36$ & $0.80$ & $0.41$ & $0.16$ & $0.36$ & $\mathbf{0.81}$ & $\mathbf{0.43}$ & $\mathbf{0.14}$ & $\mathbf{0.36}$  \\
Training 3  & $0.81$ & $0.56$ & $0.27$ & $0.33$ & $0.81$ & $0.52$ & $0.27$ & $0.33$ & $0.81$ & $0.52$ & $0.27$ & $0.33$ \\
Training 4  & $0.81$ & $0.53$ & $0.31$ & $0.25$ & $nan$ & $nan$ & $nan$ & $nan$ & $nan$ & $nan$ & $nan$ & $nan$ \\
Training 5  & $0.71$ & $0.57$ & $0.16$ & $0.35$ & $0.73$ & $0.51$ & $0.15$ & $0.36$ & $0.74$ & $0.47$ & $0.16$ & $0.36$ \\
\hline
 &  \multicolumn{12}{|c|}{MM-cVAE with latent space size $200$ $(100\times 2)$}  \\
 
 & \multicolumn{4}{c|}{epoch 100}   & \multicolumn{4}{c|}{epoch 300} & \multicolumn{4}{c|}{epoch 500} \\
 
 & \multicolumn{2}{c|}{Mnist (salient)} & \multicolumn{2}{c|}{Cifar (bg)} 
 & \multicolumn{2}{c|}{Mnist (salient)} & \multicolumn{2}{c|}{Cifar (bg)} 
 & \multicolumn{2}{c|}{Mnist (salient)} & \multicolumn{2}{c|}{Cifar (bg)}\\
 & $s_y$ $\uparrow$ & $z_y$ $\downarrow$  & $s_y$ $\downarrow$ & $z_y$ $\uparrow$ 
 & $s_y$ $\uparrow$ & $z_y$ $\downarrow$  & $s_y$ $\downarrow$ & $z_y$ $\uparrow$ 
 & $s_y$ $\uparrow$ & $z_y$ $\downarrow$  & $s_y$ $\downarrow$ & $z_y$ $\uparrow$ \\ 

Training 1  & 0.19 & 0.82 & 0.12 & 0.35 & 0.14 & 0.82 & 0.12 & 0.36 & 0.13 & 0.82 & 0.12 & 0.35 \\
Training 2  & 0.80 & 0.55 & 0.17 & 0.36 & 0.80 & 0.44 & 0.16 & 0.37 & 0.80 & 0.43 & 0.16 & 0.37  \\
Training 3  & 0.81 & 0.64 & 0.28 & 0.34 & 0.82 & 0.57 & 0.27 & 0.34 & 0.82 & 0.55 & 0.27 & 0.34 \\
Training 4  & 0.66 & 0.67 & 0.18 & 0.36 & 0.64 & 0.63 & 0.16 & 0.36 & 0.61 & 0.60 & 0.15 & 0.36 \\
Training 5  & 0.76 & 0.60 & 0.19 & 0.36 & 0.78 & 0.51 & 0.17 & 0.37 & 0.79 & 0.48 & 0.17 & 0.37 \\
\hline
 &  \multicolumn{12}{|c|}{double InfoGAN with latent space size $200$ $(100\times 2)$}  \\
 
 & \multicolumn{4}{c|}{epoch 100}   & \multicolumn{4}{c|}{epoch 300} & \multicolumn{4}{c|}{epoch 500} \\
 
 & \multicolumn{2}{c|}{Mnist (salient)} & \multicolumn{2}{c|}{Cifar (bg)} 
 & \multicolumn{2}{c|}{Mnist (salient)} & \multicolumn{2}{c|}{Cifar (bg)} 
 & \multicolumn{2}{c|}{Mnist (salient)} & \multicolumn{2}{c|}{Cifar (bg)}\\
 & $s_y$ $\uparrow$ & $z_y$ $\downarrow$  & $s_y$ $\downarrow$ & $z_y$ $\uparrow$ 
 & $s_y$ $\uparrow$ & $z_y$ $\downarrow$  & $s_y$ $\downarrow$ & $z_y$ $\uparrow$ 
 & $s_y$ $\uparrow$ & $z_y$ $\downarrow$  & $s_y$ $\downarrow$ & $z_y$ $\uparrow$ \\ 

Training 1  & 0.89 & 0.28 & 0.19 & 0.42 & 0.89 & 0.30 & 0.20 & 0.44 & 0.88 & 0.32 & 0.20 & 0.44\\
Training 2  & 0.89 & 0.29 & 0.21 & 0.41 & 0.88 & 0.31 & 0.22 & 0.43 & 0.87 & 0.32 & 0.22 & 0.44  \\
Training 3  & 0.90 & 0.28 & 0.19 & 0.42 & 0.88 & 0.32 & 0.21 & 0.44 & 0.88 & 0.32 & 0.21 & 0.44 \\
Training 4  & 0.90 & 0.29 & 0.20 & 0.41 & 0.88 & 0.30 & 0.22 & 0.43 & 0.86 & 0.32 & 0.23 & 0.43 \\
Training 5  & 0.89 & 0.28 & 0.19 & 0.41 & 0.88 & 0.30 & 0.21 & 0.44 & 0.86 & 0.32 & 0.22 & 0.43 \\
\hline
 &  \multicolumn{12}{|c|}{double InfoGAN with latent space size $128$ $(64\times 2)$ }  \\
 
 & \multicolumn{4}{c|}{epoch 100}   & \multicolumn{4}{c|}{epoch 300} & \multicolumn{4}{c|}{epoch 500} \\
 
 & \multicolumn{2}{c|}{Mnist (salient)} & \multicolumn{2}{c|}{Cifar (bg)} 
 & \multicolumn{2}{c|}{Mnist (salient)} & \multicolumn{2}{c|}{Cifar (bg)} 
 & \multicolumn{2}{c|}{Mnist (salient)} & \multicolumn{2}{c|}{Cifar (bg)}\\
 & $s_y$ $\uparrow$ & $z_y$ $\downarrow$  & $s_y$ $\downarrow$ & $z_y$ $\uparrow$ 
 & $s_y$ $\uparrow$ & $z_y$ $\downarrow$  & $s_y$ $\downarrow$ & $z_y$ $\uparrow$ 
 & $s_y$ $\uparrow$ & $z_y$ $\downarrow$  & $s_y$ $\downarrow$ & $z_y$ $\uparrow$ \\ 

Training 1  & 0.88 & 0.21 & 0.16 & 0.40 & 0.88 & 0.27 & 0.18 & 0.42 & $\mathbf{0.87}$ & $\mathbf{0.26}$ & $\mathbf{0.18}$ & $\mathbf{0.43}$ \\
Training 2  & 0.87 & 0.24 & 0.16 & 0.39 & 0.88 & 0.27 & 0.16 & 0.43 & 0.87 & 0.26 & 0.17 & 0.43  \\
Training 3  & 0.88 & 0.22 & 0.16 & 0.39 & 0.87 & 0.26 & 0.18 & 0.42 & 0.86 & 0.26 & 0.19 & 0.42\\
Training 4  & 0.87 & 0.25 & 0.17 & 0.40 & 0.88 & 0.25 & 0.19 & 0.42 & 0.87 & 0.28 & 0.19 & 0.41 \\
Training 5  & 0.88 & 0.24 & 0.15 & 0.39 & 0.87 & 0.24 & 0.17 & 0.42 & 0.86 & 0.25 & 0.19 & 0.43 \\
\hline
 &  \multicolumn{12}{|c|}{double InfoGAN with latent space size $128$ $(64\times 2)$ with CR module}  \\
 
 & \multicolumn{4}{c|}{epoch 100}   & \multicolumn{4}{c|}{epoch 300} & \multicolumn{4}{c|}{epoch 500} \\
 
 & \multicolumn{2}{c|}{Mnist (salient)} & \multicolumn{2}{c|}{Cifar (bg)} 
 & \multicolumn{2}{c|}{Mnist (salient)} & \multicolumn{2}{c|}{Cifar (bg)} 
 & \multicolumn{2}{c|}{Mnist (salient)} & \multicolumn{2}{c|}{Cifar (bg)}\\
 & $s_y$ $\uparrow$ & $z_y$ $\downarrow$  & $s_y$ $\downarrow$ & $z_y$ $\uparrow$ 
 & $s_y$ $\uparrow$ & $z_y$ $\downarrow$  & $s_y$ $\downarrow$ & $z_y$ $\uparrow$ 
 & $s_y$ $\uparrow$ & $z_y$ $\downarrow$  & $s_y$ $\downarrow$ & $z_y$ $\uparrow$ \\ 

Training 1  & $0.88$ & $0.25$ & $0.18$ & $0.42$ & $0.87$ & $0.28$ & $0.18$ & $0.43$ & $0.87$ & $0.26$ & $0.18$ & $0.43$ \\
Training 2  & $0.87$ & $0.23$ & $0.16$ & $0.40$ & $0.88$ & $0.24$ & $0.18$ & $0.43$ & $0.87$ & $0.26$ & $0.18$ & $0.42$  \\
Training 3  & $0.88$ & $0.21$ & $0.18$ & $0.40$ & $0.88$ & $0.26$ & $0.19$ & $0.43$ & $0.87$ & $0.28$ & $0.20$ & $0.43$ \\
Training 4  & $0.88$ & $0.26$ & $0.17$ & $0.39$ & $0.88$ & $0.27$ & $0.18$ & $0.42$ & $0.88$ & $0.26$ & $0.19$ & $0.42$ \\
Training 5  & $0.89$ & $0.26$ & $0.17$ & $0.40$ & $0.88$ & $0.25$ & $0.18$ & $0.42$ & $\mathbf{0.87}$ & $\mathbf{0.26}$ & $\mathbf{0.18}$ & $\mathbf{0.43}$ \\
\hline
\end{tabular}
\end{center}
\caption{Target Dataset separation on Cifar-10-MNIST for MM-cVAE and our method, with and without CR module, and for different latent space sizes. We report the results of the 5 trainings per method at different epochs. For clarity, we don't report the standard deviations, whose values are between 0.00 and 0.01. Even here, the trainings of MMc-VAE are less stable than the ones of our method, regardless of the latent dimension.}
\label{tab:target-sep-cifar2}
\end{table}

\begin{table}
    \centering
    \begin{tabular}{c|c c | c c }
    Original &  \multicolumn{2}{c}{Reconstruction}  & \multicolumn{2}{c}{Swap} \\
                        & MM-  & double & MM- & double  \\
                        & cVAE &  InfoGAN & cVAE & InfoGAN \\
        \includegraphics[width=1.7cm]{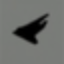} & \includegraphics[width=1.7cm]{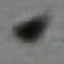} & \includegraphics[width=1.7cm]{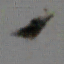} & \includegraphics[width=1.7cm]{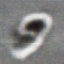} & \includegraphics[width=1.7cm]{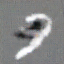} \\
        \includegraphics[width=1.7cm]{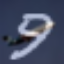} & \includegraphics[width=1.7cm]{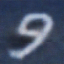} & \includegraphics[width=1.7cm]{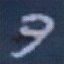} & \includegraphics[width=1.7cm]{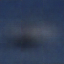} & \includegraphics[width=1.7cm]{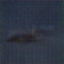} \\
        \hline \\
        \includegraphics[width=1.7cm]{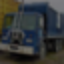} & \includegraphics[width=1.7cm]{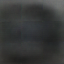} & \includegraphics[width=1.7cm]{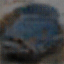} & \includegraphics[width=1.7cm]{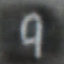} & \includegraphics[width=1.7cm]{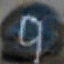} \\
        \includegraphics[width=1.7cm]{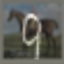} & \includegraphics[width=1.7cm]{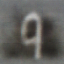} & \includegraphics[width=1.7cm]{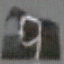} & \includegraphics[width=1.7cm]{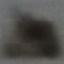} & \includegraphics[width=1.7cm]{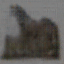} \\
        \hline \\
        \includegraphics[width=1.7cm]{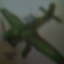} & \includegraphics[width=1.7cm]{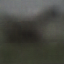} & \includegraphics[width=1.7cm]{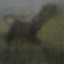} & \includegraphics[width=1.7cm]{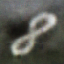} & \includegraphics[width=1.7cm]{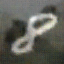} \\
        \includegraphics[width=1.7cm]{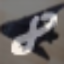} & \includegraphics[width=1.7cm]{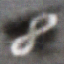} & \includegraphics[width=1.7cm]{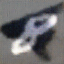} & \includegraphics[width=1.7cm]{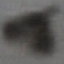} & \includegraphics[width=1.7cm]{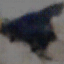} \\
        \hline \\
        \includegraphics[width=1.7cm]{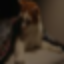} & \includegraphics[width=1.7cm]{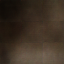} & \includegraphics[width=1.7cm]{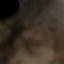} & \includegraphics[width=1.7cm]{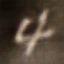} & \includegraphics[width=1.7cm]{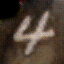} \\
        \includegraphics[width=1.7cm]{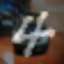} & \includegraphics[width=1.7cm]{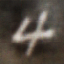} & \includegraphics[width=1.7cm]{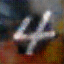} & \includegraphics[width=1.7cm]{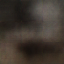} & \includegraphics[width=1.7cm]{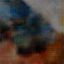} \\
    \end{tabular}
    \captionof{figure}{More examples of image reconstruction and swap with Cifar-10-MNIST dataset.}
    \label{tab:cifar-img2}
\end{table}

\begin{figure}[h!]
    \centering
    \includegraphics[width=14cm]{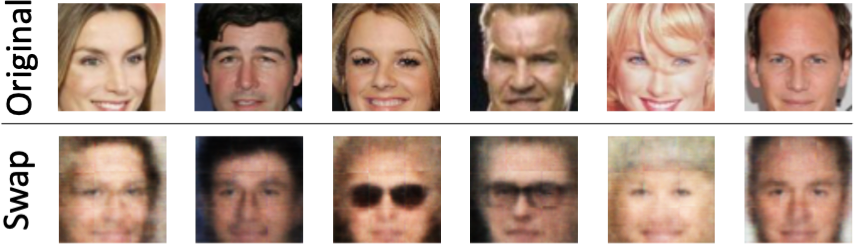}
    \caption{Swap using the cVAE method with the
CelebA with accessories dataset. We can clearly see that personal traits (which should be encoded in the common space) are lost during the swap and accessories (which should be encoded in the salient space) are not always correctly added. This could explain the poor quantitative performance of cVAE.}
    \label{fig:rebuttal}
\end{figure}

\begin{table}
\begin{center}
\begin{tabular}{|c |c |c | c | c |c | c | c | c |} 
\hline
&  \multicolumn{8}{|c|}{With CR Loss}   \\ 
& epoch 50 & epoch 100 & epoch 200 & epoch 300 & epoch 400 & epoch 500 & epoch 600 & epoch 700 \\

Training 1 & 0.334 & 0.366 & 0.366 & 0.376 & 0.394 & 0.396 & 0.398& 0.4 \\
Training 2 & 0.414 & 0.37 & 0.338 & 0.328 & 0.314 & 0.314 & 0.282 & 0.294 \\	
Training 3 & 0.258 & 0.294 & 0.25 & 0.258 & 0.222 & 0.222 & 0.218 &	0.216 \\	
Training 4 & 0.35 & 0.346 & 0.346 & 0.402 & 0.43 & 0.454 & 0.49 & \textbf{0.494} \\	
Training 5 & 0.202 & 0.202 & 0.206 & 0.216 & 0.22 & 0.222 & 0.226 & 0.24 \\
 \hline
 
&  \multicolumn{8}{|c|}{No CR Loss}   \\ 
Training 1 & 0.348 & 0.358 & 0.364 & 0.376 & 0.39 & 0.392 & 0.406 &	\textbf{0.424} \\
Training 2 & 0.348 & 0.354 & 0.372 & 0.37 & 0.378 & 0.396 & 0.398 & 0.398 \\
Training 3 & 0.326 & 0.35 &	0.354 & 0.342 &	0.334 & 0.324 & 0.306 & 0.306 \\
Training 4 & 0.292 & 0.292 & 0.288 & 0.306 & 0.316 & 0.358 & 0.348 & 0.386 \\
Training 5 & 0.306 & 0.32 & 0.318 & 0.292 & 0.304 &	0.324 & 0.334 & 0.34 \\
\hline
\end{tabular}
\end{center}
\caption{Ablation study of CR Loss on Mnist-dsprite dataset. Score indicated is fvae score}
\label{tab:fvae}
\end{table}
